# Supplementary material for: Topological surface states in strained Dirac semimetal thin films
Source: arXiv:2006.10182 ancillary file (2020-06-17)
Supplement: Supplementary file 1 [file SM.pdf]

# Supplemental Material: Topological surface states in strained $\text{Cd}_3\text{As}_2$ thin films

Pablo Villar Arribi,<sup>1</sup> Jian-Xin Zhu,<sup>2,3</sup> Timo Schumann,<sup>4</sup> Susanne Stemmer,<sup>4</sup> Anton A. Burkov,<sup>5</sup> and Olle Heinonen<sup>1,\*</sup>

<sup>1</sup>Materials Science Division, Argonne National Laboratory, Lemont, Illinois 60439, USA

<sup>2</sup>Theoretical Division, Los Alamos National Laboratory, Los Alamos, New Mexico 87545, USA

<sup>3</sup>Center for Integrated Nanotechnologies, Los Alamos National Laboratory, Los Alamos, New Mexico 87545, USA

<sup>4</sup>Materials Department, University of California, Santa Barbara, CA 93106

<sup>5</sup>Department of Physics and Astronomy, University of Waterloo, Waterloo, Ontario, Canada N2L 3G1

(Dated: June 17, 2020)

## I. DFT CALCULATIONS

For the DFT calculations, we started with the experimental lattice parameters ( $a = b = 12.633 \text{ \AA}$  and  $c = 25.427 \text{ \AA}$ ) and internal atomic positions for a centrosymmetric  $\text{Cd}_3\text{As}_2$  (Space group  $\text{I4}_1/\text{acd}$ ).<sup>1</sup> We used the pseudopotential projector-augmented wave method<sup>2</sup> implemented in the Vienna *ab initio* simulation package<sup>3,4</sup> to optimize the lattice parameters (with fixed atomic positions) for both unstrained and a strain perpendicular to the  $a$ -axis. The obtained ratios of  $b'/b$  and  $c'/c$  of the lattice parameters, together with a pre-set  $a'/a$ , were then used to rescale the experimental lattice constants, on top of which the electronic band structure was calculated with the full-potential linearized augmented plane wave (FP-LAPW) method as implemented in the Wien2k code.<sup>5</sup> A generalized gradient approximation<sup>6</sup> was used. The spin-orbital coupling was included in the FP-LAPW calculations. For the presented results, a 0.7%  $a$ -direction compressive strain was used.

### A. Fit to the DFT calculations

| Parameter                  | Unstrained | Strained |
|----------------------------|------------|----------|
| $b_1$ (eV $\text{\AA}$ )   | 0.00       | 0.2566   |
| $A$ (eV $\text{\AA}$ )     | 1.116      | 1.089    |
| $C_0$ (eV)                 | -0.0475    | 0.0113   |
| $C_1$ (eV $\text{\AA}^2$ ) | 12.50      | 12.05    |
| $C_2$ (eV $\text{\AA}^2$ ) | 13.62      | 13.13    |
| $M_0$ (eV)                 | 0.0282     | 0.0374   |
| $M_1$ (eV $\text{\AA}^2$ ) | -20.72     | -20.36   |
| $M_2$ (eV $\text{\AA}^2$ ) | -13.32     | -18.77   |

TABLE S1. Results of the fitting for the unstrained and strained cases.

## II. FITTING PROCEDURE AND RESULTS

We start by fitting the dispersion relation along different momentum directions in the Brillouin zone to the bulk band structure calculated using DFT. For these fits we do not rotate the crystal, so for the unstrained case  $\Gamma$ -Z points exactly along the crystallographic  $c$  axis and

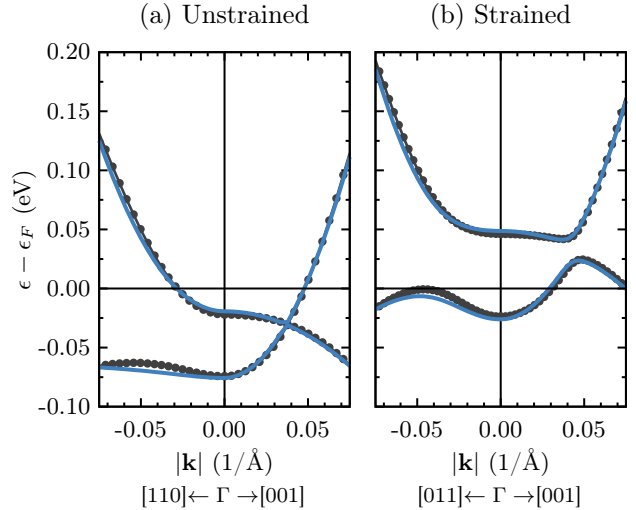

FIG. S1. Fit of four-band model  $H_1(\mathbf{k})$  given by Eq. (1) in the main text to the DFT band structure calculation along (a)  $\Gamma$ -X and  $\Gamma$ -Z directions for unstrained  $\text{Cd}_3\text{As}_2$ , and (b) along  $\Gamma$ -S and  $\Gamma$ -Z directions for a compressive strain along the  $a$ -axis of -0.7%.

$\Gamma$ -X along the  $[110]$  direction. In the case with a compressive strain of 0.7%, we fit along  $\Gamma$ -Z, this is, the  $[001]$  direction, and along  $\Gamma$ -S, which corresponds to the  $[011]$  direction. Fitting along  $\Gamma$ -Z we obtain  $M_0$ ,  $M_1$ ,  $C_0$ ,  $C_1$  and  $b_1$  in the Hamiltonian  $H_1(\mathbf{k})$  (Eq. (1) in the main text), and after we fix those values and perform the fit along  $\Gamma$ -X or  $\Gamma$ -S in order to obtain  $M_2$ ,  $C_2$ ,  $A$  and  $b_1$ . We have primarily focused on trying to reproduce the gaps and the dispersion relation close to the Dirac points, sacrificing more accuracy in the Lifshitz energies.

The results of these fittings to unstrained and strained  $\text{Cd}_3\text{As}_2$  are given in Table S1. Using our sets of parameters, we can plot the resulting dispersion relation of the model with those parameters top of the DFT calculations (Fig. S1) for unstrained and strained  $\text{Cd}_3\text{As}_2$ . These parameters reproduce quite accurately the band structure for  $|\mathbf{k}| \lesssim 0.07 \text{ \AA}^{-1}$ , and in the range of energies immediately around the Dirac points or near the gap.

### III. SOLVING FOR THE FERMI ARC STATES

Because thin films of  $\text{Cd}_3\text{As}_2$  are grown along the [112] direction, the crystallographic axes have to be rotated relative to the lab coordinate system. We can change the plane wave representation to the lab coordinate system by a rotation  $R$ . If we assume periodic boundary conditions in the  $x$  and  $y$  directions (in the lab frame), the Hamiltonian  $H_1$  yields an eigenvalue equation for energy  $E$  in  $k_z$ , given  $(k_x, k_y)$ , with eigenstates  $\alpha(E, k_x, k_y, k_z) \times e^{i(k_x x + k_y y + k_z z)}$ , where  $\alpha(E, k_x, k_y, k_z)$  is a four-component spinor in the basis  $|S_{\frac{1}{2}}, \frac{1}{2}\rangle$ ,  $|P_{\frac{3}{2}}, \frac{3}{2}\rangle$ ,  $|S_{\frac{1}{2}}, -\frac{1}{2}\rangle$ ,  $|P_{\frac{3}{2}}, -\frac{3}{2}\rangle$ , and  $k_x$ ,  $k_y$ , and  $k_z$  now refer to the lab coordinate system that is rotated with respect to the crystallographic axes with the  $z$ -axis along the [112] direction. Bulk states satisfy periodic boundary conditions in  $z$  and have real  $k_z$ , but surface states  $\psi_s(x, y, z) = \varphi(z)e^{-i(k_x x + k_y y)}$ , on the other hand, decay into the bulk and have complex-valued  $k_z \rightarrow (k_z + i\kappa)$  and  $\varphi(z) \sim e^{ik_z z - \kappa z}$  for a semi-infinite system occupying the half-space  $z < 0$ .

In general, the evanescent surface states are not admissible eigenstates as they typically do not satisfy boundary conditions, but Fermi arc states can be constructed from linear combinations of degenerate evanescent surface states such that the required boundary condition at  $z = 0$  is satisfied<sup>7</sup>. We will here use simply  $\psi(z = 0) = 0$ , which belongs to a more general class of boundary conditions<sup>7</sup>. Note that this condition cannot be satisfied by a single evanescent state, but requires at least two evanescent states degenerate in energy and with different  $\kappa$ . Formally, we construct Fermi arc states by finding evanescent states at a given energy  $E$  and momenta  $k_x, k_y$  with complex  $k_z \rightarrow k_z + i\kappa$  and  $\kappa < 0$  that satisfy the boundary condition  $\psi(z \rightarrow -\infty) = 0$ . These evanescent states, labeled  $(E, k_x, k_y, j)$  where  $j$  enumerates the degenerate states for a given  $(E, k_x, k_y)$ , are obtained by solving the characteristic equation for the full Hamilto-

nian at the given  $(E, k_x, k_y)$ . In general, the characteristic equation is an 8th-degree polynomial in  $k_z$  which will admit eight solutions,  $j = 1, 2, \dots, 8$ . These are either real or complex conjugate pairs.

Admissible Fermi arc eigenstates are formed at  $(E, k_x, k_y)$  from linear combinations of four evanescent states  $\psi_j = \alpha_{i,j} \times e^{ik_x x + ik_y y + ik_{z,j} z - \kappa_j z}$ ,  $j = 1, 2, 3, 4$ , where  $i = 1, 2, 3, 4$  enumerates the components of the four-spinor, that are necessary to satisfy the boundary condition at  $z = 0$ :  $A_1\psi_1 + A_2\psi_2 + A_3\psi_3 + A_4\psi_4 = 0$ , where  $A_j$ ,  $j = 1, \dots, 4$ , are complex numbers to be determined. This boundary condition is equivalent to  $\text{Det}[\alpha_{i,j}] = 0$ ,  $i, j = 1, 2, 3, 4$ . Note that if four degenerate spinors do not exist, the boundary condition can in general not be satisfied.

The boundary condition effectively imposes an extra relationship between  $\kappa$  and energy  $E$  for a given  $(k_x, k_y)$ . This restricts admissible solutions for  $(\kappa, E)$  to one-dimensional segments or lines in the  $(k_x, k_y)$ -plane, which are the Fermi arcs. For DSM or WSM with gapless Dirac cones and mirror symmetry such that pairs of Dirac or Weyl nodes are degenerate in energy at energy  $E_n$ , the Fermi arcs at energy  $E_n$  extend from one node to the other. In general, at energies  $E$  below or above  $E_n$ , the Fermi arcs are disconnected segments that extend from one Dirac cone to the other.

We solve the determinantal equation for the boundary condition numerically using tolerance  $\epsilon$  and  $\epsilon'$ . At a given  $(E, k_x, k_y)$  we look for evanescent states for which the imaginary parts  $\kappa$  differ by more than  $\epsilon$ . Similarly, we require that the magnitude of the determinant in the boundary condition be smaller than another  $\epsilon'$ .

In the case of a thin film, we add a second surface at  $z = -L$ . We now include complex conjugate pairs  $\pm\kappa_j$  at  $(E, k_x, k_y)$  and impose the boundary condition  $\psi(z = -L) = 0$ , in addition to  $\psi(z = 0) = 0$ , where  $\psi$  is now a linear combination of eight evanescent states. This gives a determinantal equation analogous to that for a semi-infinite thin film but for eight spinors, and with the four bottom rows of the deter

\* heinonen@anl.gov

<sup>1</sup> M. Ali, Q. Gibson, S. Jeon, A. Zhou, B. B. Yazdani, and R. Cava, *Inorg. Chem.* **53**, 4062 (2014).

<sup>2</sup> G. Kresse and D. Joubert, *Phys. Rev. B* **59**, 1758 (1999).

<sup>3</sup> G. Kresse and J. Fuethmuller, *Phys. Rev. B* **54**, 11169 (1996).

<sup>4</sup> G. Kresse and J. Hafner, *Phys. Rev. B* **48**, 13115 (1993).

<sup>5</sup> P. Blaha, K. Schwarz, F. Tran, R. Laskowski, G. K. H. Madsen, and L. Marks, *J. Chem. Phys.* **152**, 074101 (2020).

<sup>6</sup> J. Perdew, K. Burke, and M. Ernzerhof, *Phys. Rev. Lett.* **77**, 3865 (1996).

<sup>7</sup> K. Hashimoto, T. Kimura, and X. Wu, *Progress of Theoretical and Experimental Physics* **2017**, 053101 (2017).
